# Supplementary material for: Domain Generalization through Audio-Visual Relative Norm Alignment in First Person Action Recognition
Source: arXiv:2110.10101 source file (2021-10-19)
Supplement: Supplementary file 1 [file FusionStrategy.tex]

\textbf{Fusion Strategies.} %To verify the effectiveness of our design choice, we introduce a loss variant, called \textit{Hard Norm Alignment} (HNA), that induces the norms to tend to a given value arbitrarily $R$. The $R$ term is chosen after observing the range of the norms of the two modalities, and picking a value half-way between the two. 
In Table \ref{tab:ablations} we compare the \textit{late fusion} approach against the so-called \textit{mid-level fusion}, used in \cite{Kazakos_2019_ICCV}. %It consists in feeding the prediction layer with the fusion of the two modality features, i.e., concatenation.
It consists in feeding the prediction layer a concatenation of the two modality features.
%The results are shown . % Note how HNA performs worse than $\mathcal{L}_{RNA}$ in all contexts, confirming that an ``hard'' loss function constitutes in a limit. %Instead, letting the proportion between the norms of the two self-reweighting by our $\mathcal{L}_{RNA}$ leads to better results (up to $1\%$). 
As far as it concerns the mid-level fusion approach, it demonstrates to be a valid alternative in both the intra-domain (\textit{Supervised}) and cross-domain scenarios, remarking the flexibility of our method to be employed with different multi-modal fusion strategies and in all the presented settings. %It has to be noticed that RNA-Net achieves good performance also intra-domain (\textit{Supervised}).

\begin{table}
\centering

\begin{adjustbox}{width=1.0\columnwidth, margin=0ex 1ex 0ex 0ex}
\begin{tabular}{l|cccc}

\toprule\noalign{\smallskip}
\multicolumn{5}{c}{\normalsize\textsc{Fusion strategies}} \\
\noalign{\smallskip}
\cline{1-5}
\noalign{\smallskip}
  & \multicolumn{1}{c}{Supervised} & Single-DG & Multi-DG & DA\\ 
 \noalign{\smallskip} \hline
 \noalign{\smallskip}

Baseline (\textit{mid-level fusion})    & 60.18          & 40.33          & 47.61          & 40.33               \\
RNA-Net (\textit{mid-level fusion})  & 62.11          & 45.48          & 49.56          & 45.73           \\

\hline
 \noalign{\smallskip}
Baseline (\textit{late fusion})  & 59.76          & 40.93          & 44.67          & 40.93               \\

RNA-Net  (\textit{late fusion})      & \textbf{63.13} & \textbf{45.75} & \textbf{51.06} & \textbf{47.71}  \\
\bottomrule

\end{tabular}
\end{adjustbox}
\caption{Top-1 Accuracy ($\%$) of RNA-Net with two different fusion strategies, namely \textit{mid-level fusion} and \textit{late fusion}. \textbf{Bold:} highest result for each setting. }
\label{tab:ablation_}
\end{table}
